# Supplementary material for: Understanding Silent Failures in Medical Image Classification
Source: arXiv:2307.14729 source file (2023-08-22)
Supplement: Supplementary file 1 [file supplementary3056.pdf]

# A Further Results

| Dataset | Chest X-ray | | | Dermoscopy | | | | FC-Microscopy | | | Lung Nodule CT | | |
|---|---|---|---|---|---|---|---|---|---|---|---|---|---|
| Study | iid | cor | acq | iid | cor | acq | man | iid | cor | acq | iid | cor | man |
| MSR | 66.2 | 62.9 | 58.6 | 94.7 | 93.4 | 94.5 | 42.3 | 63.2 | 28.0 | 39.0 | 82.0 | 81.3 | 78.1 |
| PE | 66.2 | 62.9 | 58.6 | 94.7 | 93.4 | 94.5 | 42.3 | 63.2 | 28.0 | 39.0 | 82.0 | 81.3 | 78.1 |
| MCD-MSR | 66.8 | 63.7 | 59.9 | 94.7 | 93.4 | 94.5 | 42.4 | 63.8 | 27.3 | 39.4 | 84.4 | 83.5 | 79.1 |
| MCD-PE | 66.8 | 63.7 | 59.9 | 94.7 | 93.4 | 94.5 | 42.4 | 63.8 | 27.3 | 39.4 | 84.4 | 83.5 | 79.1 |
| MCD-EE | 66.8 | 63.7 | 59.9 | 94.7 | 93.4 | 94.5 | 42.4 | 63.8 | 27.3 | 39.4 | 84.4 | 83.5 | 79.1 |
| ConfidNet | 66.2 | 62.9 | 58.6 | 94.7 | 93.4 | 94.5 | 42.3 | 63.2 | 28.0 | 39.0 | 82.0 | 81.3 | 78.1 |
| DG-MCD-MSR | 67.5 | 63.0 | 57.8 | 94.5 | 93.6 | 94.9 | 39.8 | 71.6 | 29.3 | 39.0 | 88.1 | 83.2 | 77.9 |
| DG-RES | 66.6 | 61.8 | 55.3 | 94.5 | 93.5 | 95.0 | 39.7 | 71.1 | 30.0 | 38.8 | 87.1 | 84.6 | 76.8 |
| Devries et al. | 67.5 | 63.4 | 58.0 | 93.5 | 93.0 | 93.9 | 39.9 | 71.3 | 30.7 | 39.2 | 87.7 | 84.5 | 74.6 |

(a) Accuracy × 100 (score range: [0, 100], higher is better).

| Dataset | Chest X-ray | | | Dermoscopy | | | | FC-Microscopy | | | Lung Nodule CT | | |
|---|---|---|---|---|---|---|---|---|---|---|---|---|---|
| Study | iid | cor | acq | iid | cor | acq | man | iid | cor | acq | iid | cor | man |
| MSR | 36.5 | 33.3 | 34.3 | 87.0 | 81.8 | 62.7 | 60.3 | 62.9 | 27.3 | 37.9 | 85.0 | 82.4 | 74.2 |
| PE | 36.5 | 33.3 | 34.3 | 87.0 | 81.8 | 62.7 | 60.3 | 62.9 | 27.3 | 37.9 | 85.0 | 82.4 | 74.2 |
| MCD-MSR | 34.8 | 31.6 | 32.7 | 87.0 | 81.8 | 62.7 | 60.4 | 63.5 | 26.6 | 38.2 | 85.7 | 82.6 | 74.7 |
| MCD-PE | 34.8 | 31.6 | 32.7 | 87.0 | 81.8 | 62.7 | 60.4 | 63.5 | 26.6 | 38.2 | 85.7 | 82.6 | 74.7 |
| MCD-EE | 34.8 | 31.6 | 32.7 | 87.0 | 81.8 | 62.7 | 60.4 | 63.5 | 26.6 | 38.2 | 85.7 | 82.6 | 74.7 |
| ConfidNet | 36.5 | 33.3 | 34.3 | 87.0 | 81.8 | 62.7 | 60.3 | 62.9 | 27.3 | 37.9 | 85.0 | 82.4 | 74.2 |
| DG-MCD-MSR | 38.1 | 34.2 | 33.4 | 86.9 | 80.9 | 58.9 | 59.2 | 71.5 | 28.5 | 37.8 | 87.8 | 81.4 | 74.2 |
| DG-RES | 39.8 | 36.1 | 34.3 | 86.9 | 80.9 | 59.0 | 59.2 | 71.1 | 29.2 | 37.6 | 87.3 | 80.6 | 72.6 |
| Devries et al. | 39.2 | 35.2 | 35.6 | 88.3 | 81.8 | 59.7 | 59.2 | 71.4 | 30.1 | 38.2 | 87.2 | 81.8 | 70.7 |

(b) balanced Accuracy × 100 (score range: [0, 100], higher is better).

| Dataset | Chest X-ray | | | Dermoscopy | | | | FC-Microscopy | | | Lung Nodule CT | | |
|---|---|---|---|---|---|---|---|---|---|---|---|---|---|
| Study | iid | cor | acq | iid | cor | acq | man | iid | cor | acq | iid | cor | man |
| MSR | 79.2 | 77.0 | 77.0 | 93.5 | 91.3 | 90.6 | 55.1 | 86.6 | 78.2 | 85.8 | 78.7 | 75.8 | 70.5 |
| PE | 78.5 | 76.4 | 76.1 | 93.5 | 91.3 | 90.6 | 55.1 | 84.6 | 76.4 | 85.2 | 78.7 | 75.8 | 70.5 |
| MCD-MSR | 79.1 | 77.3 | 77.0 | 93.5 | 91.3 | 90.6 | 54.9 | 87.6 | 78.1 | 86.1 | 78.5 | 76.3 | 70.8 |
| MCD-PE | 78.5 | 76.6 | 75.9 | 93.5 | 91.3 | 90.6 | 54.9 | 85.8 | 76.5 | 85.6 | 78.5 | 76.3 | 70.8 |
| MCD-EE | 78.5 | 76.6 | 75.9 | 93.5 | 91.3 | 90.6 | 54.9 | 85.8 | 76.5 | 85.6 | 79.1 | 76.0 | 69.7 |
| ConfidNet | 79.4 | 77.3 | 77.2 | 92.8 | 90.4 | 90.5 | 51.9 | 73.9 | 62.4 | 51.8 | 82.9 | 78.6 | 65.1 |
| DG-MCD-MSR | 78.9 | 76.5 | 76.0 | 93.0 | 91.2 | 90.0 | 57.1 | 90.3 | 79.1 | 84.8 | 80.6 | 75.7 | 71.4 |
| DG-RES | 70.4 | 65.9 | 67.3 | 90.0 | 85.0 | 83.7 | 62.8 | 83.8 | 73.7 | 77.4 | 78.1 | 71.6 | 68.5 |
| Devries et al. | 78.1 | 76.7 | 76.9 | 91.8 | 89.7 | 91.1 | 63.2 | 79.6 | 59.9 | 64.4 | 76.3 | 68.0 | 62.6 |

(c) $\text{AUROC}_f$ × 100 (score range: [0, 100], higher is better).

Table 2: **Silent failure prevention benchmark results.** The coloring is normalized by column, while lighter colors depict better scores. All values denote an average of three runs. "cor" denotes the average over all corruption types and intensities levels. Similarly, "acq"/"man" denote averages over all acquisition/manifestation shifts per dataset. "iid" denotes scenarios without distribution shifts.

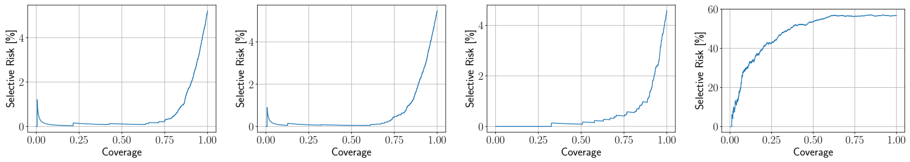


(a) I.i.d. (b) Corruption Shift (c) Acquisition Shift (d) Manif. Shift

Fig. 3: **Exemplary Risk-Coverage Curves of the Dermoscopy dataset.** Shown is the selective risk over the coverage of one classifier per shift. Filtering is done based on Maximum Softmax Response.

# B Dataset and Training Parameters

(a) **Summary of image corruptions strengths.** Brighter/Darker are pixel-wise multipliers, Motion Blur is described by the size of the line filter, Elastic Transformation is described by the amplitude of the applied Gaussian filter, Gaussian noise is described by its variance.

| Dataset | Brighter | | Darker | | Motion Blur | | Elastic | | Gaussian Noise | |
|---|---|---|---|---|---|---|---|---|---|---|
| | + | ++ | + | ++ | + | ++ | + | ++ | + | ++ |
| Chest X-ray | 1.125 | 1.25 | 0.875 | 0.750 | 5 | 10 | 10 | 20 | 20 | 40 |
| Dermoscopy | 1.250 | 1.50 | 0.500 | 0.250 | 10 | 30 | 40 | 60 | 20 | 100 |
| FC-Microscopy | 1.125 | 1.25 | 0.875 | 0.750 | 10 | 30 | 40 | 60 | 5 | 10 |
| Lung Nodule CT | 1.400 | 1.70 | 0.600 | 0.300 | 5 | 10 | 10 | 20 | 80 | 160 |

(b) **Summary of tuned and CSF specific hyperparameters.** init-lr: Initial learning rate, wd: weight decay, batch: batch size, DV-eps: total training epochs when using the training scheme for DeVries et al., DG-eps: number of epochs for DeepGamblers training stages, CN-eps: number of epochs for ConfidNet training stages.

| Dataset | init-lr | wd | batch | DV-eps | DG-eps | CN-eps | Budget | Reward |
|---|---|---|---|---|---|---|---|---|
| Chest X-ray | 5e-4 | 1e-4 | 96 | 30 | 30+10 | 40+10+10 | 0.3 | 10 |
| Dermoscopy | 3e-5 | 0.0 | 16 | 15 | 15+5 | 20+5+5 | 0.3 | 10 |
| FC-Microscopy | 1.5e-4 | 1e-5 | 70 | 90 | 90+30 | 160+40+40 | 0.3 | 10 |
| Lung Nodule CT | 1.5e-4 | 0.1 | 512 | 45 | 45+15 | 45+15+15 | 0.3 | 20 |

(c) **Summary of class prevalences for Dermoscopy datasets.**

| **Dermoscopy** | Tot. w/o Bar. | Bar. | w/o MSKCC | MSKCC | S.c. iid | S.c. ood |
|---|---|---|---|---|---|---|
| Benign | 0.95 | 0.94 | 0.98 | 0.92 | 0.98 | 0.82 | 0.77 |
| Malignant | 0.05 | 0.06 | 0.02 | 0.08 | 0.02 | 0.18 | 0.23 |

(d) **Summary of class prevalences for Chest X-ray datasets.**

| **Chest X-ray** | Tot. w/o Nih14 | Nih14 | w/o CheXpert | CheXpert |
|---|---|---|---|---|
| No Finding | 0.51 | 0.46 | 0.72 | 0.63 | 0.31 |
| Cardiomegaly | 0.07 | 0.07 | 0.02 | 0.08 | 0.03 |
| Edema | 0.04 | 0.06 | 0.01 | 0.03 | 0.09 |
| Consolidation | 0.02 | 0.02 | 0.02 | 0.02 | 0.02 |
| Pneumonia | 0.03 | 0.03 | 0.01 | 0.04 | 0.02 |
| Atelectasis | 0.08 | 0.08 | 0.08 | 0.09 | 0.07 |
| Pneumothorax | 0.05 | 0.04 | 0.04 | 0.03 | 0.07 |
| Pleural Effusion | 0.20 | 0.22 | 0.08 | 0.08 | 0.37 |

(e) **Summary of class prevalences for Lung Nodule CT datasets.**

| **Lung Nodule** | Tot. | Cal. iid | Cal. ood | Spi. iid | Spi. ood | Tex. iid | Tex. ood |
|---|---|---|---|---|---|---|---|
| Benign | 0.25 | 0.33 | 0.00 | 0.15 | 0.80 | 0.19 | 0.27 |
| Malignant | 0.75 | 0.67 | 1.00 | 0.85 | 0.20 | 0.81 | 0.73 |

Table 3: **Additional training and dataset details.**
